# Supplementary material for: YASO: A Targeted Sentiment Analysis Evaluation Dataset for Open-Domain Reviews
Source: arXiv:2012.14541 source file (2021-09-13)
Supplement: Supplementary file 1 [file appendix_main.tex]

% This must be in the first 5 lines to tell arXiv to use pdfLaTeX, which is strongly recommended.
\pdfoutput=1

%%%%%%%%start EMNLP

% In particular, the hyperref package requires pdfLaTeX in order to break URLs across lines.

\documentclass[11pt]{article}

% Remove the "review" option to generate the final version.
\usepackage[review]{resources/emnlp2021}

% Standard package includes
\usepackage{times}
\usepackage{latexsym}

% For proper rendering and hyphenation of words containing Latin characters (including in bib files)
\usepackage[T1]{fontenc}
% For Vietnamese characters
% \usepackage[T5]{fontenc}
% See https://www.latex-project.org/help/documentation/encguide.pdf for other character sets

% This assumes your files are encoded as UTF8
\usepackage[utf8]{inputenc}

% This is not strictly necessary, and may be commented out,
% but it will improve the layout of the manuscript,
% and will typically save some space.
\usepackage{microtype}

%%%%%%%%%%%% end EMNLP

% Standard package includes
\usepackage{graphicx}
\graphicspath{ {./} }
\usepackage{url}
\usepackage{xspace}
\usepackage{comment}
\usepackage{multirow}
\usepackage{booktabs} % quality tables in latex
\usepackage{subfig}
\usepackage{soul}
\newcommand\rurl[1]{%
  \href{https://#1}{\nolinkurl{#1}}%
}

% If the title and author information does not fit in the area allocated, uncomment the following
%
%\setlength\titlebox{<dim>}
%
% and set <dim> to something 5cm or larger.

\title{\YasoName: A Targeted Sentiment Analysis Evaluation Dataset\\for Open-Domain Reviews\\[0.2cm]
\supp}

% Author information can be set in various styles:
% For several authors from the same institution:
% \author{Author 1 \and ... \and Author n \\
%         Address line \\ ... \\ Address line}
% if the names do not fit well on one line use
%         Author 1 \\ {\bf Author 2} \\ ... \\ {\bf Author n} \\
% For authors from different institutions:
% \author{Author 1 \\ Address line \\  ... \\ Address line
%         \And  ... \And
%         Author n \\ Address line \\ ... \\ Address line}
% To start a seperate ``row'' of authors use \AND, as in
% \author{Author 1 \\ Address line \\  ... \\ Address line
%         \AND
%         Author 2 \\ Address line \\ ... \\ Address line \And
%         Author 3 \\ Address line \\ ... \\ Address line}

\author{Matan Orbach, Orith Toledo-Ronen, Artem Spector,\\
        {\bf Ranit Aharonov, Yoav Katz, Noam Slonim} \\
IBM Research \\
\texttt{\{matano, oritht, artems, katz, noams\}@il.ibm.com}\\ \texttt{ranit.aharonov2@ibm.com}\\
}

\input{commands}

\begin{document}
\maketitle

\section{Contents}
This \supp contains:
\begin{enumerate}
    \item Examples of (i) sentences with the corresponding annotated targets and their sentiments, and (ii) sentences in which clusters containing a relatively large number of valid targets were annotated.
    \item Examples of review domains that have annotated reviews included in \YasoName. 
    %MO12 \item A survey of the evaluation datasets used in a sample of recent papers.
    \item Detailed benchmark results, reporting additional evaluation metrics.
    \item The annotation guidelines for each of the two annotation phases.
\end{enumerate}

\input{appendices/appendix}

\bibliography{main}

\end{document}
